# Supplementary material for: Run Time Analysis for Random Local Search on Generalized Majority Functions
Source: arXiv:2204.12770 source file (2022-09-26)
Supplement: Supplementary file 1 [file additional_commands.tex]

% Lets one create labels in starred math environments.
\newcommand\numberthis{\addtocounter{equation}{1}\tag{\theequation}}


% Indicator function
\newcommand*{\indicator}[1]{\mathOrText{\mathds{1}{(#1)}}}

% Random process
\DeclareDocumentCommand{\randomProcess}{o}
{%
    \mathOrText{X\IfNoValueTF{#1}{}{_{#1}}}%
}

% Transformed process
\DeclareDocumentCommand{\transformedProcess}{o}
{%
    \mathOrText{Y\IfNoValueTF{#1}{}{_{#1}}}%
}

% Transformed process
\DeclareDocumentCommand{\transformedProcessOther}{o}
{%
    \mathOrText{Z\IfNoValueTF{#1}{}{_{#1}}}%
}

% Transformed process
\DeclareDocumentCommand{\randomProcessOther}{o}
{%
    \mathOrText{Y\IfNoValueTF{#1}{}{_{#1}}}%
}

% Another transformed process
\DeclareDocumentCommand{\randomProcessThird}{o}
{%
    \mathOrText{Z\IfNoValueTF{#1}{}{_{#1}}}%
}

% Filtration
\DeclareDocumentCommand{\filtration}{o}
{%
    \mathOrText{\mathcal{F}\IfNoValueTF{#1}{}{_{#1}}}%
}

% Other filtration
\DeclareDocumentCommand{\filtrationOther}{o}
{%
    \mathOrText{\mathcal{G}\IfNoValueTF{#1}{}{_{#1}}}%
}

% Other filtration
\DeclareDocumentCommand{\filtrationSecondOther}{o}
{%
    \mathOrText{\mathcal{G}'\IfNoValueTF{#1}{}{_{#1}}}%
}

% Individual
\DeclareDocumentCommand{\individual}{o}
{%
    \mathOrText{\boldsymbol{x}\IfNoValueTF{#1}{}{^{(#1)}}}%
}

% Another individual
\DeclareDocumentCommand{\individualOther}{o}
{%
    \mathOrText{\boldsymbol{y}\IfNoValueTF{#1}{}{^{(#1)}}}%
}

% Third individual
\DeclareDocumentCommand{\individualThird}{o}
{%
    \mathOrText{\boldsymbol{z}\IfNoValueTF{#1}{}{^{(#1)}}}%
}

% Difference of time points
\DeclareDocumentCommand{\difference}{o}
{%
    \mathOrText{\Delta\IfNoValueTF{#1}{}{_{#1}}}%
}

% Sequence of run time points
\DeclareDocumentCommand{\runTimePoints}{m}
{%
    \mathOrText{N_{\textrm{#1}}}%
}

% Sequence of return time points
\DeclareDocumentCommand{\returnTimePoints}{m}
{%
    \mathOrText{M_{\textrm{#1}}}%
}

\DeclareDocumentCommand{\returnTimePointsStart}{o}
{%
    \mathOrText{R_{\IfNoValueTF{#1}{}{#1}}}%
}

\DeclareDocumentCommand{\returnTimePointsEnd}{o}
{%
    \mathOrText{O_{\IfNoValueTF{#1}{}{#1}}}%
}

% Sequence of retries
\DeclareDocumentCommand{\retry}{o}
{%
    \mathOrText{M\IfNoValueTF{#1}{}{_{#1}}}%
}

% A command for defining a sequence. The first parameter is the symbol of the sequence, the second (optional) parameter is its index, the third (optional) parameter is the index set, and the fourth (optional) parameter is the size of the brackets. Note that brackets are only shown if the second argument is not empty.
\DeclareDocumentCommand{\sequence}{m o o o}%
{%
    \mathOrText{\IfNoValueTF{#2}{#1}{\IfEmptyTF{#2}{#1}{\IfNoValueTF{#4}{\left}{#4}(#1_{#2}\IfNoValueTF{#4}{\right}{#4})_{#2 \in #3}}}}%
}

% Various math commands
\newcommand*{\timePoint}{\mathOrText{t}}
\newcommand*{\timePointOther}{\mathOrText{s}}
\newcommand*{\stoppingTime}{\mathOrText{T}}
\newcommand*{\stoppingTimeOther}{\mathOrText{S}}
\newcommand*{\stoppingTimeThird}{\mathOrText{U}}
\newcommand*{\drift}{\mathOrText{\delta}}
\newcommand*{\defeq}{\mathOrText{\coloneqq}}
\newcommand*{\eqdef}{\mathOrText{\eqqcolon}}
\newcommand*{\plateauDistance}{\mathOrText{r}}
\newcommand*{\basisRLS}{\mathOrText{\lambda}}
\newcommand*{\potentialFunction}{\mathOrText{g}}
\newcommand*{\runTimeBound}{\mathOrText{R}}
\newcommand*{\returnTimeBound}{\mathOrText{M}}
\newcommand*{\runTimeSet}{\mathOrText{\mathcal{R}}}
\newcommand*{\returnTimeSet}{\mathOrText{\mathcal{M}}}
\newcommand*{\myAlgorithm}{\mathOrText{A}}
\newcommand*{\probabilityOfSuccessAfterFailure}{\mathOrText{p}}
\newcommand*{\probabilityOfImmediateSuccess}{\mathOrText{\probabilityOfSuccessAfterFailure_0}}
\newcommand*{\myIndex}{\mathOrText{i}}
\newcommand*{\majority}{\mathOrText{\textsc{Majority}^{(1)}_{0}}}
\newcommand*{\basisRLSNumerator}{\mathOrText{a}}
\newcommand*{\onemax}{\textsc{OneMax}\xspace}
\newcommand*{\jump}{\textsc{Jump}\xspace}
\newcommand*{\initialization}{\mathOrText{D}}
\newcommand*{\RExtended}{\mathOrText{\overline{\R}}}
\newcommand*{\eventForRestart}{\mathOrText{L}}

% Names and stuff
\DeclareDocumentCommand{\plateau}{o}
{%
    \mathOrText{\textsc{HasMajority}\IfNoValueTF{#1}{}{_{#1}}}%
}
\DeclareDocumentCommand{\asymmetricPlateau}{o}
{%
    \mathOrText{\textsc{Majority}\IfNoValueTF{#1}{}{_{#1}}}%
}
\DeclareDocumentCommand{\rls}{o}
{%
    RLS\IfNoValueF{#1}{$_{#1}$}\xspace%
}
\DeclareDocumentCommand{\onePlusOneEA}{o}
{%
    \mathOrText{(1 + 1)~\textrm{EA}\IfNoValueF{#1}{_{#1}}}%
}

% The mutation operator
\DeclareDocumentCommand{\mutation}{o}
{%
    \mathOrText{\phi\IfNoValueTF{#1}{}{_{#1}}}%
}

% Labels
% Defines an optional argument for labels named ›case‹ that signals that cleveref should name the respective reference ›case‹ instead of its actual name.
\crefname{case}{case}{cases}
\creflabelformat{case}{#2{\upshape#1}#3}
