# Supplementary material for: Run Time Analysis for Random Local Search on Generalized Majority Functions
Source: arXiv:2204.12770 source file (2022-09-26)
Supplement: Supplementary file 2 [file additional_packages.tex]

\usepackage{balance}
\usepackage{bbold}
